# Supplementary material for: Practical and Consistent Estimation of f-Divergences
Source: arXiv:1905.11112 source file (2019-10-24)
Supplement: Supplementary file 1 [file proof_others.tex]

\subsection{Proof that various $f$-divergences are admissible}

\paragraph{$\chi^2$:}
Taking $f(x) = x^2 - 1$, we have that
\begin{align*}
    f'(x) &= 2x \\
    \implies f_0(x) &= x^2 - 2x \\
    \implies f'_0(x) &= 2(x - 1) \\
    \implies f'^2_0(x) &= 4(x-1)^2 \\
\end{align*}
and hence $f$ is admissible.

\paragraph{Hellinger Distance:}
Taking $f(x) = f_0(x) = (1-\sqrt{x})^2$, we have that
\begin{align*}
    f'_0(x) &= 1- \frac{1}{\sqrt{x}} \\
    \implies f'^2_0(x) &= 1- \frac{2}{\sqrt{x}} + \frac{1}{x}
\end{align*}

\paragraph{Total Variation:}
Taking $f(x) = f_0(x) = |x-1|$, we have that 
\begin{align*}
    f'_0(x) = \begin{cases} 1 & x>1 \\ -1 & x<1 \\ 
    0 & x=1
    \end{cases}
\end{align*}
where $f'_0(1)=0$ is a sub-gradient of $f_0$ at $x=1$. 
Thus
\begin{align*}
    f'^2_0(x) \leq h(x) = 1
\end{align*}
and so $f$ is admissible.

\paragraph{$\alpha$-divergence:}

Taking $f(x) = f_0(x) = \frac{4 \left(1 - x^{\frac{1+\alpha}{2}}\right)}{1-\alpha^2}$ we have that
\begin{align*}
    f'_0(x) = \frac{2 x^{\frac{\alpha - 1}{2}}}{1-\alpha}
\end{align*}
